# Supplementary material for: CADIS: Handling Cluster-skewed Non-IID Data in Federated Learning with Clustered Aggregation and Knowledge DIStilled Regularization
Source: arXiv:2302.10413 source file (2023-04-15)
Supplement: Supplementary file 1 [file supplementary.tex]

\documentclass[10pt, conference, letterpaper]{IEEEtran}
\usepackage{amsmath,amsfonts}
\usepackage{array}
\usepackage[caption=false,font=normalsize,labelfont=sf,textfont=sf]{subfig}
\usepackage{textcomp}
\usepackage{stfloats}
\usepackage{url}
\usepackage{verbatim}
\usepackage{graphicx}
\usepackage{cite}
\hyphenation{op-tical net-works semi-conduc-tor IEEE-Xplore}

\usepackage{xcolor}
\usepackage[colorlinks = true,
            linkcolor = blue,
            urlcolor  = blue,
            citecolor = blue,
            anchorcolor = blue]{hyperref}
\usepackage{algorithm}
\usepackage{algpseudocode}
\usepackage{todonotes}
\usepackage{soul}
\usepackage{multirow}
\usepackage{booktabs}
\begin{document}
\title{Appendix: Artifact Description for paper 9766 \\CADIS: Handling Cluster-skewed Non-IID Data in Federated Learning with Clustered Aggregation and Knowledge Distilled Regularization}

\maketitle
\begin{IEEEkeywords}
Federated learning, non-IID data, clustering, knowledge distillation, regularization, aggregation.
\end{IEEEkeywords}
\input{reproduce}
\bibliographystyle{IEEEtran}
\bibliography{main}
\end{document}
